# Supplementary material for: How to Pare a Pair: Topology Control and Pruning in Intertwined Complex Networks
Source: arXiv:1909.06114 source file (2020-08-13)
Supplement: Supplementary file 1 [file appendix_c.tex]

\section{Limit case of uncoupled flow networks}\label{apx:uncoupled_networks}
	 From the rescaled ODE set of two coupled networks we may easily reproduce the uncoupled case for the two networks by setting $\lambda_1=\lambda_1'=0$. With focus on just one network we have the radii adaptation,
	    \alg{\partd{h}\rho_e & =\lambda_0\brc{ \rho_e^2\mean{\LP\Phi^2_e}-\lambda_2}\rho_e \label{eq:ode}\\
	   \text{with } \mean{\LP\Phi^2_e} & =\sum_{jk}\vc{\alpha}^e_{jk}\brc{\vc{U}_{jk}+\lambda_3\vc{V}_{jk}}\nonumber}
		which resembles the gradient flow driven optimization model proposed in the original Hu-Cai model \cite{Hu:2013io} in combination with the flow fluctuation notation proposed in \cite{Corson:2010ee}. We calculate the adaptation of simple cubic networks with a single corner source node (sinks otherwise) for a systematic scan of $\lambda_2$, $\lambda_3$, see Figure \ref{fig:scale} and \ref{fig:dynamics}. In particular we can show that in agreement with \cite{Hu:2013io} only an increase in the flow to fluctuation ratio $\lambda_3$ results in an increase of nullity and that the continuous transition observed is independent of the systems effective volume penalty $\lambda_2$, see Figure \ref{fig:scale}. The system's transition is logarithmic for $\lambda_3>1$ and saturates for large $\lambda_3$, as was shown in the main body of this study. This transition is qualitatively conserved for all other periodic lattices, i.e. fcc, bcc and diamond lattice follow the same transition type.
  		
  		\begin{figure}[H]
  		\centering
  		%\subfloat[]{\label{fig:scale_a} \includegraphics[scale=0.25]{./Figures/appendix/snapshot01_L02.png}}
			 %\subfloat[]{
			\includegraphics[scale=1.]{./Figures_Supplement/mean_21178355_21178354_21178353/sweep_eval/NULLITY_MATRIX.pdf}
			 %}
%			\caption{Network plots and state diagram for $n=216$, $m=540$: \subR{fig:scale_a} Simple cubic lattice as primary plexus. \subR{fig:scale_b}Systematic $\bra{\lambda_2,\lambda_3}$ scan displays no dependency of $\lambda_2$ }
\caption{Network nullity state diagram for $\bra{\lambda_2,\lambda_3}$: No dependency of volume penalty $\lambda_2$, onset of fluctuation induced loops is controlled by rate of fluctuation $\lambda_3$ }
\label{fig:scale} 
		\end{figure}
		\begin{figure}[H]
		\centering
		 \subfloat[]{\label{fig:prune_1} \includegraphics[scale=.6]{./Figures_Supplement/21511081/N_216E_540_500000x0.0001mode_pointleaf_c1_1.0_c2_0.1/eval/network_3d_plot.pdf}}
			\subfloat[]{\label{fig:radius_time_1} \includegraphics[scale=1.]{./Figures_Supplement/21511081/N_216E_540_500000x0.0001mode_pointleaf_c1_1.0_c2_0.1/eval/radius_time.pdf}}\\
 			 \subfloat[]{\label{fig:prune_2} \includegraphics[scale=.6]{./Figures_Supplement/21511081/N_216E_540_500000x0.0001mode_pointleaf_c1_1.0_c2_10.0/eval/network_3d_plot.pdf}}
 			\subfloat[]{\label{fig:radius_time_2} \includegraphics[scale=1.]{./Figures_Supplement/21511081/N_216E_540_500000x0.0001mode_pointleaf_c1_1.0_c2_10.0/eval/radius_time.pdf}}\\
 			\subfloat[]{\label{fig:prune_3} \includegraphics[scale=.6]{./Figures_Supplement/21511081/N_216E_540_500000x0.0001mode_pointleaf_c1_1.0_c2_1000.0/eval/network_3d_plot.pdf}}
 			\subfloat[]{\label{fig:radius_time_3} \includegraphics[scale=1.]{./Figures_Supplement/21511081/N_216E_540_500000x0.0001mode_pointleaf_c1_1.0_c2_1000.0/eval/radius_time.pdf}}
\caption{
Adaptation dynamics and pruned network skeletons: \subR{fig:prune_1}$+$\subR{fig:radius_time_1} Tree-like configuration for $\lambda_2=\lambda_3=1$. \subR{fig:prune_2}$+$\subR{fig:radius_time_2} Onset of reticulation for $\lambda_2=1$ and $\lambda_3=10$.\subR{fig:prune_3}$+$\subR{fig:radius_time_3} Saturation of fluctuation induced loops for $\lambda_2=1$ and $\lambda_3=1000$. The edge thickness is representative for the relative tube radius $\rho$. Sinks are marked as blue dots, the source as large red circle.}\label{fig:dynamics} 
		\end{figure}
	The actual dynamics and pruned structures are represented for several sample parameters in Fig. \ref{fig:dynamics}. Fluctuation induced pruning into spanning trees usually takes place on shorter time-scales then their reticulated pendants and displays less avalanche-like events of a edge radii suddenly collapsing. \\
Nevertheless, there is also a quantitative variation of the final nullity, depending on the total network size, see Figure \ref{fig:size_a}. How then is the trajectory dependent on the actual system size? An answer could be given by looking into the fluctuation generating machinery which manifests the positive feedback in \eqref{eq:ode}. Adding up $\vc{U}$ and $\vc{V}$ and resorting the terms around $\lambda_3$, we rewrite $\mean{\LP\Phi^2_e}$ as,
		  \alg{\mean{\LP\Phi^2_e} & =\sum_{jk}\vc{\alpha}^e_{jk}\vc{W}_{jk}\bra{\lambda_3} \label{eq:solution_mean}\\
		 \text{with } \vc{W}_{jk} & = \bra{1+\delta_{0j}\delta_{0k}-\delta_{0j}-\delta_{0k}}+\lambda_3\bra{\delta_{jk}-\delta_{0j}\delta_{0k}}\nonumber\\& +\bra{n-1}\bra{\bra{n+1}\delta_{0j}\delta_{0k}-\delta_{0j}-\delta_{0k}}\brc{1+\frac{\lambda_3}{n-1}}}
		  By introducing further abbreviations to improve readability we rewrite \eqref{eq:solution_mean} as,		
		    \alg{\vc{W}_{jk} &=\vc{w}_{0,jk}+\vc{w}_{1,jk}\lambda_3+\vc{w}_{2,jk}h\bra{\lambda_3 ,n} \label{eq:slution_mean_abbreviation}
		    \\ \text{ with }\vc{w}_{0,jk} & = \bra{1+\delta_{0j}\delta_{0k}-\delta_{0j}-\delta_{0k}}\nonumber\\ \vc{w}_{1,jk} & =\bra{\delta_{jk}-\delta_{0j}\delta_{0k}}\nonumber\\ \vc{w}_{2,jk} & =\bra{n-1}\brc{\bra{n+1}\delta_{0j}\delta_{0k}-\delta_{0j}-\delta_{0k}}\nonumber\\ h\bra{\lambda_3 ,n} & =1+\frac{\lambda_3}{n-1}\nonumber}
Hence we have $h\bra{\lambda_3,n}\longrightarrow 1$, for large networks with small fluctuations $\lambda_3 \ll n$, so  the solution in \eqref{eq:slution_mean_abbreviation} becomes,
 		  \g{\vc{W}_{jk}\approx \bra{\vc{w}_{0,jk}+\vc{w}_{2,jk}}+\vc{w}_{1,jk}\lambda_3 \label{eq:size_flow_ratio}}
 		  This impact on the (positive) feedback terms suggest a size dependent change in the overall network structure. Though we can't exclude the possibility of other finite size effects, such as the ratio of surface (nodes with a degree smaller than the maximal possible for the lattice) to volume nodes(nodes with maximum degree). We can observe the transition to follow a logarithmic relation for any network size (node number $n$),
		\g{\varrho_n\bra{\lambda_3}=a_n\cdot lg\bra{\lambda_3-\lambda_3^n} + b_n}
		From fitting the trajectories in \ref{fig:size_a} one can quantitatively see that the transition curves converge with increasing $n$ at given $\lambda_3$, suggesting our approximation to be a plausible cause. 
		\begin{figure}
		\centering
			 \subfloat[]{\label{fig:size_a} \includegraphics[scale=1.]{./Figures_Supplement/mean_loglaw.pdf}}\\
			 \subfloat[]{\label{fig:size_b} \includegraphics[scale=1.]{./Figures_Supplement/x0_loglaw.pdf}}
			 \subfloat[]{\label{fig:size_c} \includegraphics[scale=1.]{./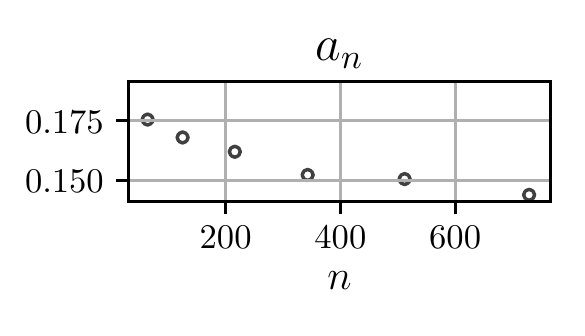}}
			 \subfloat[]{\label{fig:size_d} \includegraphics[scale=1.]{./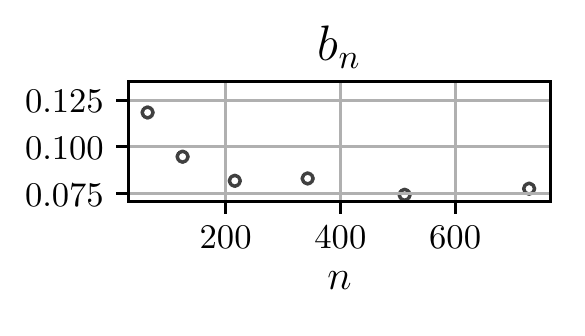}}
			\caption{Size dependency for nullity transition in cubic lattice: \subR{fig:size_a} Different network sizes(amount of nodes) and logarithmic fits for $\lambda_2=1$.\subR{fig:size_b} -\subR{fig:size_d} Size dependecies o thef fit parameters $\lambda_3^n$, $a_n$ and $b_n$} 	\label{fig:size} 
		\end{figure}
