# Supplementary material for: How to Pare a Pair: Topology Control and Pruning in Intertwined Complex Networks
Source: arXiv:1909.06114 source file (2020-08-13)
Supplement: Supplementary file 2 [file appendix_d.tex]

\section{Coupled flow networks}\label{apx:coupled_networks}
In the following we collected the entirety of numeric results for both networks spanning our system, including an overview of the respective adaptation dynamics during the the optimization and plots of pruned network skeletons starting from cubic, diamond and Laves graph topologies. 
%We begin with a commented results section of the 'dual' cubic graphs. Further we find qualitative similar results for other graph topologies such as the 'dual' diamond graphs and the 'dual' Laves graphs.  The edge affiliation definition from cubic networks will be redefined at this point: Instead of affiliating edges penetrating faces we define distance criterion stating that edges should have a distance $d$ for given network topology to be affiliated with each other, see table \ref{tab:dist_crit}. 
%\begin{table}[h]
%\centering
%\begin{tabular}{ l | l | l}
%	Topology & distance (in units of the constructed graph's node positions) & max. number of affiliations per edge\\ \hline
%	dual cubic & $0.5$ & $4$\\
%	dual diamond&	$\sqrt{2}$& $6$\\
%	dual Laves &	$\sqrt{14}$ & $8$
%\end{tabular}
%\caption{Specifics for intertwined graph topologies of the triply periodic surfaces P, D and G}
%\label{tab:dist_crit}
%\end{table}
\subsection{Complementary cubic lattices}
 In Figure \ref{fig:bilayer} we present the nullity transition for the intertwined cubic networks, displaying yet again the retardation of  the transitions onset for increasing coupling $\lambda_1$. The dual cubic structure was generated by first repeating a unit cell (consisting of points $\bra{0,0,0}$, $\bra{0,0,1}$, $\bra{1,0,0}$, $\bra{0,1,0}$,$\bra{1,1,1}$, $\bra{1,0,1}$, $\bra{0,1,1}$, $\bra{1,1,0}$, connecting those pairs of relative distance $\delta=1$) periodically with the three translation vectors $\vc{a}=i*\bra{1,0,0}$, $\vc{b}=j*\bra{0,1,0}$, $\vc{c}=k*\bra{0,0,1}$ with $i,j,k \in\mathbb{Z} $. The second network is acquired by copying the first structure and shifting it by $\vc{t}=\bra{0.5,0.5,0.5}$.
  \begin{figure}[H]
 	\subfloat[]{\label{fig:bilayer_time_1}	\begin{minipage}[h]{5cm}
 	 \includegraphics[scale=.7]{./Figures_Supplement/21506711/N_275E_450_200000x5e-06mode_pointleaf_alpha_0.1_beta_1.0/eval/combined_radius_time.pdf}
 	 \end{minipage}
 }
 \subfloat[]{\label{fig:bilayer_final_1} 
 	\begin{minipage}[h]{2cm}
 		 \includegraphics[scale=.35]{./Figures_Supplement/21506711/N_275E_450_200000x5e-06mode_pointleaf_alpha_0.1_beta_1.0/eval/network_3d_plot_0.pdf}\\
 		 \includegraphics[scale=.35]{./Figures_Supplement/21506711/N_275E_450_200000x5e-06mode_pointleaf_alpha_0.1_beta_1.0/eval/network_3d_plot_1.pdf}
\end{minipage}} \hfill
 		\subfloat[]{\label{fig:bilayer_time_2}	\begin{minipage}[h]{5cm} \includegraphics[scale=.7]{./Figures_Supplement/21506711/N_275E_450_200000x1e-09mode_pointleaf_alpha_0.1_beta_100000000.0/eval/combined_radius_time.pdf}
 		 \end{minipage}}
 	\subfloat[]{\label{fig:bilayer_final_2}\begin{minipage}{2cm}
 		 \includegraphics[scale=.35]{./Figures_Supplement/21506711/N_275E_450_200000x1e-09mode_pointleaf_alpha_0.1_beta_100000000.0/eval/network_3d_plot_0.pdf}\\
 		 \includegraphics[scale=.35]{./Figures_Supplement/21506711/N_275E_450_200000x1e-09mode_pointleaf_alpha_0.1_beta_100000000.0/eval/network_3d_plot_1.pdf}
\end{minipage} }\\
 		\subfloat[]{\label{fig:bilayer_time_3}	\begin{minipage}[h]{5cm} \includegraphics[scale=.7]{./Figures_Supplement/21506711/N_275E_450_200000x1e-09mode_pointleaf_alpha_1000.0_beta_100000000.0/eval/combined_radius_time.pdf} \end{minipage}}
 	\subfloat[]{\label{fig:bilayer_final_3} \begin{minipage}{2cm}
 		 \includegraphics[scale=.35]{./Figures_Supplement/21506711/N_275E_450_200000x1e-09mode_pointleaf_alpha_1000.0_beta_100000000.0/eval/network_3d_plot_0.pdf}\\
 		 \includegraphics[scale=.35]{./Figures_Supplement/21506711/N_275E_450_200000x1e-09mode_pointleaf_alpha_1000.0_beta_100000000.0/eval/network_3d_plot_1.pdf}
\end{minipage} }\hfill
 		\subfloat[]{\label{fig:bilayer_time_4}	\begin{minipage}[h]{5cm} \includegraphics[scale=.7]{./Figures_Supplement/21506711/N_275E_450_200000x5e-06mode_pointleaf_alpha_1000.0_beta_1.0/eval/combined_radius_time.pdf} \end{minipage}}
 	\subfloat[]{\label{fig:bilayer_final_4} \begin{minipage}{2cm}
 		 \includegraphics[scale=.35]{./Figures_Supplement/21506711/N_275E_450_200000x5e-06mode_pointleaf_alpha_1000.0_beta_1.0/eval/network_3d_plot_0.pdf}\\
 		 \includegraphics[scale=.35]{./Figures_Supplement/21506711/N_275E_450_200000x5e-06mode_pointleaf_alpha_1000.0_beta_1.0/eval/network_3d_plot_1.pdf}
\end{minipage} }
 	\caption{Adaptation Dynamics for a complimentary cubic lattice system and pruned network skeletons. The edge thickness is representative for the relative tube radius $\rho$. \subR{fig:bilayer_time_1}$+$\subR{fig:bilayer_final_1} $\lambda_1=1$, $\lambda_3=0.1$ \subR{fig:bilayer_time_2}$+$\subR{fig:bilayer_final_2} $\lambda_1=10^8$, $\lambda_3=0.1$ \subR{fig:bilayer_time_3}$+$\subR{fig:bilayer_final_3} $\lambda_1=10^8$, $\lambda_3=10^3$ \subR{fig:bilayer_time_4}$+$\subR{fig:bilayer_final_4} $\lambda_1=1$, $\lambda_3=10^3$}\label{fig:bilayer_dynamics}
 \end{figure}
\begin{figure}[H]
	\hspace{-1cm}\subfloat[]{\label{fig:bilayer_aux_3} \includegraphics[scale=1.]{./Figures_Supplement/21572518/sweep_eval/NULLITY_FIT_0.pdf}}
 	\subfloat[]{\label{fig:bilayer_aux_4} \includegraphics[scale=1.]{./Figures_Supplement/21572518/sweep_eval/NULLITY_FIT_1.pdf}}\\
 	\subfloat[]{	\label{fig:bilayer_nullity_c1} \includegraphics[scale=1.]{./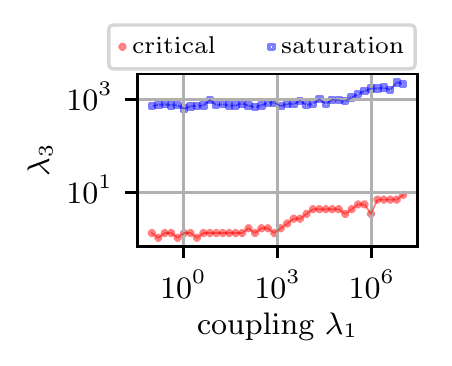}}
 	\subfloat[]{	\label{fig:bilayer_nullity_c2} \includegraphics[scale=1.]{./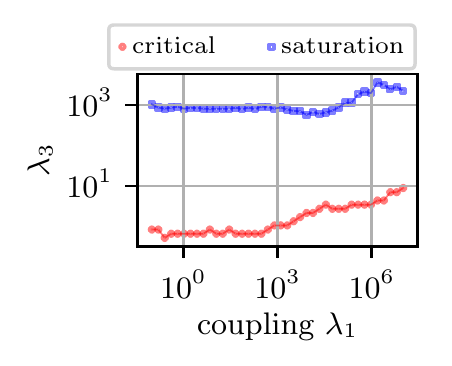}}
 	\caption{Numeric results and analysis of  for a complimentary cubic lattice system: \subR{fig:bilayer_aux_3}+\subR{fig:bilayer_aux_4} Continuous, logarithmic nullity transition in dependency for various coupling $\lambda_1$. Increasing coupling breaks down fluctuation induced nullity.  \subR{fig:bilayer_nullity_c1}$+$\subR{fig:bilayer_nullity_c2} Saturation (blue, squares) and critical values (red circles) in dependency of coupling $\lambda_1$.}\label{fig:bilayer}
\end{figure}
Phenomenologically, the transition resembles an asymmetrical sigmoidal for $\lambda_3 > \lambda_c$, whose saturation value, steepness and x-offset are functions of $\lambda_1$.  Note that, though qualitatively similar, the curves development for increasing $\lambda_1$ is different in the two networks. In particular we observe a significant change of the saturation onset in the second network, see Figure \ref{fig:bilayer_nullity_c1}, \ref{fig:bilayer_nullity_c2}. Next we have listed the systematic $\lambda_1$, $\lambda_3$ of the final stationary state after pruning. In Figure \ref{fig:bilayer_nullity_c1}, \ref{fig:bilayer_nullity_c2} we present the nullity state diagrams as well as the respective outline of their transition zones: first spanning trees, second the onset of redundancy and third the onset of saturation. The colored, dashed boundaries of these zones represent the curves' fits from Figure \ref{fig:bilayer_nullity_c1} and \ref{fig:bilayer_nullity_c1}.
%In Figure \ref{fig:bilayer_aux_3},\ref{fig:bilayer_aux_4} we show dissipation diagrams, presenting the the systems power dissipation ${D=\sum_e \kappa_{ee} \mean{\LP \Phi_e^2}}$ for each network. Note that the systems dissipation is not significantly increased  by an increase of the coupling until extreme values for $\lambda_1$ are reached.  In Figure \ref{fig:bilayer_aux_5},\ref{fig:bilayer_aux_6} we show the networks volume calculated as $V=\sum_e \rho_e^2$ (vessel segments are modelled as cylindrical tubes). We observe here that the tube system collapses for $\lambda_1 > 10^5$ in opposition to the fluctuation induced increase of the systems volume.
In Figure \ref{fig:bilayer_dynamics} we present the numeric results for the systems radii dynamics and plots of the pruned networks for various parameter combinations. An increase in $\lambda_1=\frac{b\bra{\varepsilon-1}}{\pi l \eta L^{\varepsilon+1}}\bra{\frac{\mu}{L^3}}^{-2}$ is decreasing the final radius size $\rho_e$, as it incorporates not only the strength of the repulsive potential but can also be seen as an increase off the systems density by bringing the edges closer to each other.
\subsection{Complementary diamond lattices}
The next segment will contain the gathered results for dual diamond structures where we see the results to be very similar to the cubic structure. The dual structure was generated by first repeating a unit cell (consisting of points $\bra{0,0,0}$,$\bra{0.5,0.5,0.5}$, $\bra{1,0,1}$, $\bra{0,1,1}$, $\bra{1,1,0}$ , connecting those pairs of relative distance $\delta=\sqrt{3}/2$) periodically with the three translation vectors $\vc{a}=i*\bra{1,0,0}$, $\vc{b}=j*\bra{0,1,0}$, $\vc{c}=k*\bra{0,0,1}$ with $i,j,k \in\mathbb{Z}$ and $(i+j+k) mod 2=0$. The second network is acquired by copying the first structure and shifting it by $\vc{t}=\bra{1,1,1}$.
\begin{figure}[H]
  
 	\subfloat[]{\label{fig:bilayer_time_1}	\begin{minipage}[h]{5cm}
 	 \includegraphics[scale=.7]{./Figures_Supplement/22809199/N_141E_214_250000x1e-06mode_pointleaf_alpha_0.1_beta_1.0/eval/combined_radius_time.pdf}
 	 \end{minipage}
 }
 \subfloat[]{\label{fig:bilayer_final_1} 
 	\begin{minipage}[h]{2cm}
 		 \includegraphics[scale=.35]{./Figures_Supplement/22809199/N_141E_214_250000x1e-06mode_pointleaf_alpha_0.1_beta_1.0/eval/network_3d_plot_0.pdf}\\
 		 \includegraphics[scale=.35]{./Figures_Supplement/22809199/N_141E_214_250000x1e-06mode_pointleaf_alpha_0.1_beta_1.0/eval/network_3d_plot_1.pdf}
\end{minipage}} \hfill
 		\subfloat[]{\label{fig:bilayer_time_2}	\begin{minipage}[h]{5cm} \includegraphics[scale=.7]{./Figures_Supplement/22809199/N_141E_214_200000x1e-09mode_pointleaf_alpha_0.1_beta_100000000.0/eval/combined_radius_time.pdf}
 		 \end{minipage}}
 	\subfloat[]{\label{fig:bilayer_final_2}\begin{minipage}{2cm}
 		 \includegraphics[scale=.35]{./Figures_Supplement/22809199/N_141E_214_200000x1e-09mode_pointleaf_alpha_0.1_beta_100000000.0/eval/network_3d_plot_0.pdf}\\
 		 \includegraphics[scale=.35]{./Figures_Supplement/22809199/N_141E_214_200000x1e-09mode_pointleaf_alpha_0.1_beta_100000000.0/eval/network_3d_plot_1.pdf}
\end{minipage} }\\
 		\subfloat[]{\label{fig:bilayer_time_3}	\begin{minipage}[h]{5cm} \includegraphics[scale=.7]{./Figures_Supplement/22809199/N_141E_214_200000x1e-09mode_pointleaf_alpha_1000.0_beta_100000000.0/eval/combined_radius_time.pdf} \end{minipage}}
 	\subfloat[]{\label{fig:bilayer_final_3} \begin{minipage}{2cm}
 		 \includegraphics[scale=.35]{./Figures_Supplement/22809199/N_141E_214_200000x1e-09mode_pointleaf_alpha_1000.0_beta_100000000.0/eval/network_3d_plot_0.pdf}\\
 		 \includegraphics[scale=.35]{./Figures_Supplement/22809199/N_141E_214_200000x1e-09mode_pointleaf_alpha_1000.0_beta_100000000.0/eval/network_3d_plot_1.pdf}
\end{minipage} }\hfill
 		\subfloat[]{\label{fig:bilayer_time_4}	\begin{minipage}[h]{5cm} \includegraphics[scale=.7]{./Figures_Supplement/22809199/N_141E_214_250000x1e-06mode_pointleaf_alpha_1000.0_beta_1.0/eval/combined_radius_time.pdf} \end{minipage}}
 	\subfloat[]{\label{fig:bilayer_final_4} \begin{minipage}{2cm}
 		 \includegraphics[scale=.35]{./Figures_Supplement/22809199/N_141E_214_250000x1e-06mode_pointleaf_alpha_1000.0_beta_1.0/eval/network_3d_plot_0.pdf}\\
 		 \includegraphics[scale=.35]{./Figures_Supplement/22809199/N_141E_214_250000x1e-06mode_pointleaf_alpha_1000.0_beta_1.0/eval/network_3d_plot_1.pdf}
\end{minipage} }
 	\caption{Adaptation Dynamics for a complimentary diamond graph system and pruned network skeletons. The edge thickness is representative for the relative tube radius $\rho$. \subR{fig:bilayer_time_1}$+$\subR{fig:bilayer_final_1} $\lambda_1=1$, $\lambda_3=0.1$ \subR{fig:bilayer_time_2}$+$\subR{fig:bilayer_final_2} $\lambda_1=10^8$, $\lambda_3=0.1$ \subR{fig:bilayer_time_3}$+$\subR{fig:bilayer_final_3} $\lambda_1=10^8$, $\lambda_3=10^3$ \subR{fig:bilayer_time_4}$+$\subR{fig:bilayer_final_4} $\lambda_1=1$, $\lambda_3=10^3$}\label{fig:bilayer_dynamics}
 \end{figure}
\begin{figure}[H]
	\hspace{-1cm}\subfloat[]{\label{fig:D_3} \includegraphics[scale=1.]{./Figures_Supplement/22926223/sweep_eval/NULLITY_FIT_0.pdf}}
 	\subfloat[]{\label{fig:D_4} \includegraphics[scale=1.]{./Figures_Supplement/22926223/sweep_eval/NULLITY_FIT_1.pdf}}\\
 	\subfloat[]{	\label{fig:D_nullity_c1} \includegraphics[scale=1.]{./Figures_Supplement/22926223/sweep_eval/fit_critical_saturation_0.pdf}}
 	\subfloat[]{	\label{fig:D_nullity_c2} \includegraphics[scale=1.]{./Figures_Supplement/22926223/sweep_eval/fit_critical_saturation_1.pdf}}
 	\caption{Numeric results and analysis for a complimentary diamond graph system: \subR{fig:bilayer_aux_3}+\subR{fig:bilayer_aux_4} Continuous, logarithmic nullity transition in dependency for various coupling $\lambda_1$. Increasing coupling breaks down fluctuation induced nullity.  \subR{fig:bilayer_nullity_c1}$+$\subR{fig:bilayer_nullity_c2} Saturation (blue, squares) and critical values (red circles) in dependency of coupling $\lambda_1$.}\label{fig:bilayer_D}
\end{figure}
% \begin{figure}[H]
% \vspace{-2cm}
% 	\subfloat[]{\label{fig:bilayer_D_1} \includegraphics[scale=1.]{./Figures_Supplement/22926223/sweep_eval/NULLITY_MATRIX_0_extended.pdf}}
% 	\subfloat[]{\label{fig:bilayer_D_2} \includegraphics[scale=1.]{./Figures_Supplement/22926223/sweep_eval/NULLITY_MATRIX_1_extended.pdf}}\\
% 	\subfloat[]{\label{fig:bilayer_D_3} \includegraphics[scale=1.]{./Figures_Supplement/22926223/sweep_eval/DISS_MATRIX_0.pdf}}
% 	\subfloat[]{\label{fig:bilayer_D_4} \includegraphics[scale=1.]{./Figures_Supplement/22926223/sweep_eval/DISS_MATRIX_1.pdf}}\\
% 	\subfloat[]{\label{fig:bilayer_D_5} \includegraphics[scale=1.]{./Figures_Supplement/22926223/sweep_eval/VOL_MATRIX_0.pdf}}
% 	\subfloat[]{\label{fig:bilayer_D_6} \includegraphics[scale=1.]{./Figures_Supplement/22926223/sweep_eval/VOL_MATRIX_1.pdf}}
% 	\caption{Numeric results and analysis for a 'dual' diamond graph system: \subR{fig:bilayer_aux_1}$+$\subR{fig:bilayer_aux_2}Nullity $\varrho$ state diagrams with borders of the transition zones plotted as dashed lines( red $=$ onset of nullity transition, black $=$ onset of saturation) \subR{fig:bilayer_aux_3}$+$\subR{fig:bilayer_aux_4}Dissipation diagrams, coupling $\lambda_1$ and fluctuation $\lambda_3$ are not majorly affecting the systems dissipation \subR{fig:bilayer_aux_5}$+$\subR{fig:bilayer_aux_6} Volume diagrams, we observe an increase of V for increased $\lambda_3$, a collapse is occuring for increased $\lambda_1$.}\label{fig:bilayer2}
% \end{figure}
\subsection{Complementary Laves graphs}
The next segment will contain the gathered results for dual Laves structures where we see the results as well to be very similar to the cubic structure. The dual structure was generated by first repeating a unit cell (consisting of points $\bra{0,0,0}$,$\bra{1,1,0}$, $\bra{1,2,1}$, $\bra{0,3,1}$, $\bra{2,2,2}$, $\bra{3,3,2}$, $\bra{3,0,3}$ , $\bra{2,1,3}$, connecting those pairs of relative distance $\delta=\sqrt{2}$) periodically with the three translation vectors $\vc{a}=i*\bra{4,0,0}$, $\vc{b}=j*\bra{0,4,0}$, $\vc{c}=k*\bra{0,0,4}$ with $i,j,k \in\mathbb{Z}$. The second network is acquired mirroring in order to create the opposing chirality of the first structure, i.e. $\vc{a}\rightarrow -\vc{a}$, and shifting it by $\vc{t}=\bra{3,2,0}$.
\begin{figure}[H]

 	\subfloat[]{\label{fig:bilayer_time_1}	\begin{minipage}[h]{5cm}
 	 \includegraphics[scale=.7]{./Figures_Supplement/22809169/N_206E_259_250000x1e-06mode_pointleaf_alpha_0.1_beta_1.0/eval/combined_radius_time.pdf}
 	 \end{minipage}
 }
 \subfloat[]{\label{fig:bilayer_final_1} 
 	\begin{minipage}[h]{2cm}
 		 \includegraphics[scale=.35]{./Figures_Supplement/22809169/N_206E_259_250000x1e-06mode_pointleaf_alpha_0.1_beta_1.0/eval/network_3d_plot_0.pdf}\\
 		 \includegraphics[scale=.35]{./Figures_Supplement/22809169/N_206E_259_250000x1e-06mode_pointleaf_alpha_0.1_beta_1.0/eval/network_3d_plot_1.pdf}
\end{minipage}} \hfill
 		\subfloat[]{\label{fig:bilayer_time_2}	\begin{minipage}[h]{5cm} \includegraphics[scale=.7]{./Figures_Supplement/22809169/N_206E_259_200000x1e-09mode_pointleaf_alpha_0.1_beta_100000000.0/eval/combined_radius_time.pdf}
 		 \end{minipage}}
 	\subfloat[]{\label{fig:bilayer_final_2}\begin{minipage}{2cm}
 		 \includegraphics[scale=.35]{./Figures_Supplement/22809169/N_206E_259_200000x1e-09mode_pointleaf_alpha_0.1_beta_100000000.0/eval/network_3d_plot_0.pdf}\\
 		 \includegraphics[scale=.35]{./Figures_Supplement/22809169/N_206E_259_200000x1e-09mode_pointleaf_alpha_0.1_beta_100000000.0/eval/network_3d_plot_1.pdf}
\end{minipage} }\\
 		\subfloat[]{\label{fig:bilayer_time_3}	\begin{minipage}[h]{5cm} \includegraphics[scale=.7]{./Figures_Supplement/22809169/N_206E_259_200000x1e-09mode_pointleaf_alpha_1000.0_beta_100000000.0/eval/combined_radius_time.pdf} \end{minipage}}
 	\subfloat[]{\label{fig:bilayer_final_3} \begin{minipage}{2cm}
 		 \includegraphics[scale=.35]{./Figures_Supplement/22809169/N_206E_259_200000x1e-09mode_pointleaf_alpha_1000.0_beta_100000000.0/eval/network_3d_plot_0.pdf}\\
 		 \includegraphics[scale=.35]{./Figures_Supplement/22809169/N_206E_259_200000x1e-09mode_pointleaf_alpha_1000.0_beta_100000000.0/eval/network_3d_plot_1.pdf}
\end{minipage} }\hfill
 		\subfloat[]{\label{fig:bilayer_time_4}	\begin{minipage}[h]{5cm} \includegraphics[scale=.7]{./Figures_Supplement/22809169/N_206E_259_250000x1e-06mode_pointleaf_alpha_1000.0_beta_1.0/eval/combined_radius_time.pdf} \end{minipage}}
 	\subfloat[]{\label{fig:bilayer_final_4} \begin{minipage}{2cm}
 		 \includegraphics[scale=.35]{./Figures_Supplement/22809169/N_206E_259_250000x1e-06mode_pointleaf_alpha_1000.0_beta_1.0/eval/network_3d_plot_0.pdf}\\
 		 \includegraphics[scale=.35]{./Figures_Supplement/22809169/N_206E_259_250000x1e-06mode_pointleaf_alpha_1000.0_beta_1.0/eval/network_3d_plot_1.pdf}
\end{minipage} }
 	\caption{Adaptation Dynamics for a complimentary Laves graph system and pruned network skeletons. The edge thickness is representative for the relative tube radius $\rho$. \subR{fig:bilayer_time_1}$+$\subR{fig:bilayer_final_1} $\lambda_1=1$, $\lambda_3=0.1$ \subR{fig:bilayer_time_2}$+$\subR{fig:bilayer_final_2} $\lambda_1=10^8$, $\lambda_3=0.1$ \subR{fig:bilayer_time_3}$+$\subR{fig:bilayer_final_3} $\lambda_1=10^8$, $\lambda_3=10^3$ \subR{fig:bilayer_time_4}$+$\subR{fig:bilayer_final_4} $\lambda_1=1$, $\lambda_3=10^3$}\label{fig:bilayer_dynamics}
 \end{figure}
\begin{figure}[H]
	\hspace{-1cm}\subfloat[]{\label{fig:D_3} \includegraphics[scale=1.]{./Figures_Supplement/22868425/sweep_eval/NULLITY_FIT_0.pdf}}
 	\subfloat[]{\label{fig:D_4} \includegraphics[scale=1.]{./Figures_Supplement/22868425/sweep_eval/NULLITY_FIT_1.pdf}}\\
 	\subfloat[]{	\label{fig:D_nullity_c1} \includegraphics[scale=1.]{./Figures_Supplement/22868425/sweep_eval/fit_critical_saturation_0.pdf}}
 	\subfloat[]{	\label{fig:D_nullity_c2} \includegraphics[scale=1.]{./Figures_Supplement/22868425/sweep_eval/fit_critical_saturation_1.pdf}}
 	\caption{Numeric results and analysis for a 'dual' Laves graph system: \subR{fig:bilayer_aux_3}+\subR{fig:bilayer_aux_4} Continuous, logarithmic nullity transition in dependency for various coupling $\lambda_1$. Increasing coupling breaks down fluctuation induced nullity.  \subR{fig:bilayer_nullity_c1}$+$\subR{fig:bilayer_nullity_c2} Saturation (blue, squares) and critical values (red circles) in dependency of coupling $\lambda_1$.}\label{fig:bilayer_D}
\end{figure}
% \begin{figure}[H]
% \vspace{-2cm}
% 	\subfloat[]{\label{fig:bilayer_D_1} \includegraphics[scale=1.]{./Figures_Supplement/22868425/sweep_eval/NULLITY_MATRIX_0_extended.pdf}}
% 	\subfloat[]{\label{fig:bilayer_D_2} \includegraphics[scale=1.]{./Figures_Supplement/22868425/sweep_eval/NULLITY_MATRIX_1_extended.pdf}}\\
% 	\subfloat[]{\label{fig:bilayer_D_3} \includegraphics[scale=1.]{./Figures_Supplement/22868425/sweep_eval/DISS_MATRIX_0.pdf}}
% 	\subfloat[]{\label{fig:bilayer_D_4} \includegraphics[scale=1.]{./Figures_Supplement/22868425/sweep_eval/DISS_MATRIX_1.pdf}}\\
% 	\subfloat[]{\label{fig:bilayer_D_5} \includegraphics[scale=1.]{./Figures_Supplement/22868425/sweep_eval//VOL_MATRIX_0.pdf}}
% 	\subfloat[]{\label{fig:bilayer_D_6} \includegraphics[scale=1.]{./Figures_Supplement/22868425/sweep_eval/VOL_MATRIX_1.pdf}}
% 	\caption{Numeric results and analysis for a 'dual' Laves graph system: \subR{fig:bilayer_aux_1}$+$\subR{fig:bilayer_aux_2}Nullity $\varrho$ state diagrams with borders of the transition zones plotted as dashed lines( red $=$ onset of nullity transition, black $=$ onset of saturation) \subR{fig:bilayer_aux_3}$+$\subR{fig:bilayer_aux_4}Dissipation diagrams, coupling $\lambda_1$ and fluctuation $\lambda_3$ are not majorly affecting the systems dissipation \subR{fig:bilayer_aux_5}$+$\subR{fig:bilayer_aux_6} Volume diagrams, we observe an increase of V for increased $\lambda_3$, a collapse is occuring for increased $\lambda_1$.}\label{fig:bilayer2}
% \end{figure}
