# Supplementary material for: How to Pare a Pair: Topology Control and Pruning in Intertwined Complex Networks
Source: arXiv:1909.06114 source file (2020-08-13)
Supplement: Supplementary file 3 [file SI.tex]

\pdfoutput=1
\documentclass[9pt,twoside,lineno]{pnas-new}
% Use the lineno option to display guide line numbers if required.
\input{./packages}
\input{./macros}
\templatetype{pnassupportinginfo}
% \readytosubmit %% Uncomment this line before submitting, so that the instruction page is removed.

\title{How to Pare a Pair: Topology Control and Pruning in Intertwined Complex Networks.}
\author{Felix Kramer, Carl Modes}
\correspondingauthor{Carl Modes.\\E-mail: modes@mpi-cbg.de}

\begin{document}
%\maketitle
%% Adds the main heading for the SI text. Comment out this line if you do not have any supporting information text.
\SItext

\input{./Sections_Supplement/appendix_a}
\newpage
\input{./Sections_Supplement/appendix_b}
\newpage
\section{Limit case of uncoupled flow networks}\label{apx:uncoupled_networks}
	 From the rescaled ODE set of two coupled networks we may easily reproduce the uncoupled case for the two networks by setting $\lambda_1=\lambda_1'=0$. With focus on just one network we have the radii adaptation,
	    \alg{\partd{h}\rho_e & =\lambda_0\brc{ \rho_e^2\mean{\LP\Phi^2_e}-\lambda_2}\rho_e \label{eq:ode}\\
	   \text{with } \mean{\LP\Phi^2_e} & =\sum_{jk}\vc{\alpha}^e_{jk}\brc{\vc{U}_{jk}+\lambda_3\vc{V}_{jk}}\nonumber}
		which resembles the gradient flow driven optimization model proposed in the original Hu-Cai model \cite{Hu:2013io} in combination with the flow fluctuation notation proposed in \cite{Corson:2010ee}. We calculate the adaptation of simple cubic networks with a single corner source node (sinks otherwise) for a systematic scan of $\lambda_2$, $\lambda_3$, see Figure \ref{fig:scale} and \ref{fig:dynamics}. In particular we can show that in agreement with \cite{Hu:2013io} only an increase in the flow to fluctuation ratio $\lambda_3$ results in an increase of nullity and that the continuous transition observed is independent of the systems effective volume penalty $\lambda_2$, see Figure \ref{fig:scale}. The system's transition is logarithmic for $\lambda_3>1$ and saturates for large $\lambda_3$, as was shown in the main body of this study. This transition is qualitatively conserved for all other periodic lattices, i.e. fcc, bcc and diamond lattice follow the same transition type.
  		
  		\begin{figure}[H]
  		\centering
  		%\subfloat[]{\label{fig:scale_a} \includegraphics[scale=0.25]{./Figures/appendix/snapshot01_L02.png}}
			 %\subfloat[]{
			\includegraphics[scale=1.]{./Figures_Supplement/mean_21178355_21178354_21178353/sweep_eval/NULLITY_MATRIX.pdf}
			 %}
%			\caption{Network plots and state diagram for $n=216$, $m=540$: \subR{fig:scale_a} Simple cubic lattice as primary plexus. \subR{fig:scale_b}Systematic $\bra{\lambda_2,\lambda_3}$ scan displays no dependency of $\lambda_2$ }
\caption{Network nullity state diagram for $\bra{\lambda_2,\lambda_3}$: No dependency of volume penalty $\lambda_2$, onset of fluctuation induced loops is controlled by rate of fluctuation $\lambda_3$ }
\label{fig:scale} 
		\end{figure}
		\begin{figure}[H]
		\centering
		 \subfloat[]{\label{fig:prune_1} \includegraphics[scale=.6]{./Figures_Supplement/21511081/N_216E_540_500000x0.0001mode_pointleaf_c1_1.0_c2_0.1/eval/network_3d_plot.pdf}}
			\subfloat[]{\label{fig:radius_time_1} \includegraphics[scale=1.]{./Figures_Supplement/21511081/N_216E_540_500000x0.0001mode_pointleaf_c1_1.0_c2_0.1/eval/radius_time.pdf}}\\
 			 \subfloat[]{\label{fig:prune_2} \includegraphics[scale=.6]{./Figures_Supplement/21511081/N_216E_540_500000x0.0001mode_pointleaf_c1_1.0_c2_10.0/eval/network_3d_plot.pdf}}
 			\subfloat[]{\label{fig:radius_time_2} \includegraphics[scale=1.]{./Figures_Supplement/21511081/N_216E_540_500000x0.0001mode_pointleaf_c1_1.0_c2_10.0/eval/radius_time.pdf}}\\
 			\subfloat[]{\label{fig:prune_3} \includegraphics[scale=.6]{./Figures_Supplement/21511081/N_216E_540_500000x0.0001mode_pointleaf_c1_1.0_c2_1000.0/eval/network_3d_plot.pdf}}
 			\subfloat[]{\label{fig:radius_time_3} \includegraphics[scale=1.]{./Figures_Supplement/21511081/N_216E_540_500000x0.0001mode_pointleaf_c1_1.0_c2_1000.0/eval/radius_time.pdf}}
\caption{
Adaptation dynamics and pruned network skeletons: \subR{fig:prune_1}$+$\subR{fig:radius_time_1} Tree-like configuration for $\lambda_2=\lambda_3=1$. \subR{fig:prune_2}$+$\subR{fig:radius_time_2} Onset of reticulation for $\lambda_2=1$ and $\lambda_3=10$.\subR{fig:prune_3}$+$\subR{fig:radius_time_3} Saturation of fluctuation induced loops for $\lambda_2=1$ and $\lambda_3=1000$. The edge thickness is representative for the relative tube radius $\rho$. Sinks are marked as blue dots, the source as large red circle.}\label{fig:dynamics} 
		\end{figure}
	The actual dynamics and pruned structures are represented for several sample parameters in Fig. \ref{fig:dynamics}. Fluctuation induced pruning into spanning trees usually takes place on shorter time-scales then their reticulated pendants and displays less avalanche-like events of a edge radii suddenly collapsing. \\
Nevertheless, there is also a quantitative variation of the final nullity, depending on the total network size, see Figure \ref{fig:size_a}. How then is the trajectory dependent on the actual system size? An answer could be given by looking into the fluctuation generating machinery which manifests the positive feedback in \eqref{eq:ode}. Adding up $\vc{U}$ and $\vc{V}$ and resorting the terms around $\lambda_3$, we rewrite $\mean{\LP\Phi^2_e}$ as,
		  \alg{\mean{\LP\Phi^2_e} & =\sum_{jk}\vc{\alpha}^e_{jk}\vc{W}_{jk}\bra{\lambda_3} \label{eq:solution_mean}\\
		 \text{with } \vc{W}_{jk} & = \bra{1+\delta_{0j}\delta_{0k}-\delta_{0j}-\delta_{0k}}+\lambda_3\bra{\delta_{jk}-\delta_{0j}\delta_{0k}}\nonumber\\& +\bra{n-1}\bra{\bra{n+1}\delta_{0j}\delta_{0k}-\delta_{0j}-\delta_{0k}}\brc{1+\frac{\lambda_3}{n-1}}}
		  By introducing further abbreviations to improve readability we rewrite \eqref{eq:solution_mean} as,		
		    \alg{\vc{W}_{jk} &=\vc{w}_{0,jk}+\vc{w}_{1,jk}\lambda_3+\vc{w}_{2,jk}h\bra{\lambda_3 ,n} \label{eq:slution_mean_abbreviation}
		    \\ \text{ with }\vc{w}_{0,jk} & = \bra{1+\delta_{0j}\delta_{0k}-\delta_{0j}-\delta_{0k}}\nonumber\\ \vc{w}_{1,jk} & =\bra{\delta_{jk}-\delta_{0j}\delta_{0k}}\nonumber\\ \vc{w}_{2,jk} & =\bra{n-1}\brc{\bra{n+1}\delta_{0j}\delta_{0k}-\delta_{0j}-\delta_{0k}}\nonumber\\ h\bra{\lambda_3 ,n} & =1+\frac{\lambda_3}{n-1}\nonumber}
Hence we have $h\bra{\lambda_3,n}\longrightarrow 1$, for large networks with small fluctuations $\lambda_3 \ll n$, so  the solution in \eqref{eq:slution_mean_abbreviation} becomes,
 		  \g{\vc{W}_{jk}\approx \bra{\vc{w}_{0,jk}+\vc{w}_{2,jk}}+\vc{w}_{1,jk}\lambda_3 \label{eq:size_flow_ratio}}
 		  This impact on the (positive) feedback terms suggest a size dependent change in the overall network structure. Though we can't exclude the possibility of other finite size effects, such as the ratio of surface (nodes with a degree smaller than the maximal possible for the lattice) to volume nodes(nodes with maximum degree). We can observe the transition to follow a logarithmic relation for any network size (node number $n$),
		\g{\varrho_n\bra{\lambda_3}=a_n\cdot lg\bra{\lambda_3-\lambda_3^n} + b_n}
		From fitting the trajectories in \ref{fig:size_a} one can quantitatively see that the transition curves converge with increasing $n$ at given $\lambda_3$, suggesting our approximation to be a plausible cause. 
		\begin{figure}
		\centering
			 \subfloat[]{\label{fig:size_a} \includegraphics[scale=1.]{./Figures_Supplement/mean_loglaw.pdf}}\\
			 \subfloat[]{\label{fig:size_b} \includegraphics[scale=1.]{./Figures_Supplement/x0_loglaw.pdf}}
			 \subfloat[]{\label{fig:size_c} \includegraphics[scale=1.]{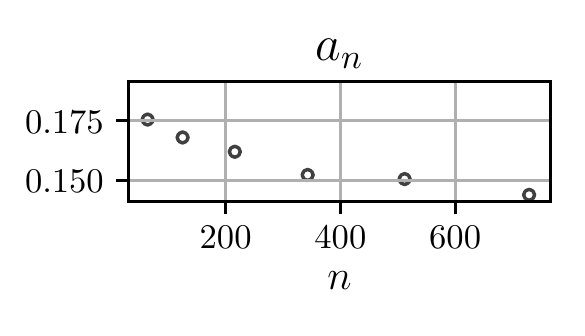}}
			 \subfloat[]{\label{fig:size_d} \includegraphics[scale=1.]{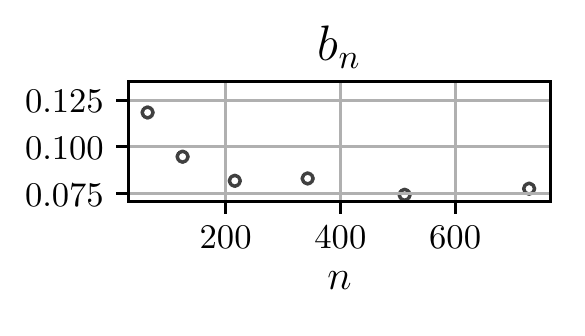}}
			\caption{Size dependency for nullity transition in cubic lattice: \subR{fig:size_a} Different network sizes(amount of nodes) and logarithmic fits for $\lambda_2=1$.\subR{fig:size_b} -\subR{fig:size_d} Size dependecies o thef fit parameters $\lambda_3^n$, $a_n$ and $b_n$} 	\label{fig:size} 
		\end{figure}

\newpage
\section{Coupled flow networks}\label{apx:coupled_networks}
In the following we collected the entirety of numeric results for both networks spanning our system, including an overview of the respective adaptation dynamics during the the optimization and plots of pruned network skeletons starting from cubic, diamond and Laves graph topologies. 
%We begin with a commented results section of the 'dual' cubic graphs. Further we find qualitative similar results for other graph topologies such as the 'dual' diamond graphs and the 'dual' Laves graphs.  The edge affiliation definition from cubic networks will be redefined at this point: Instead of affiliating edges penetrating faces we define distance criterion stating that edges should have a distance $d$ for given network topology to be affiliated with each other, see table \ref{tab:dist_crit}. 
%\begin{table}[h]
%\centering
%\begin{tabular}{ l | l | l}
%	Topology & distance (in units of the constructed graph's node positions) & max. number of affiliations per edge\\ \hline
%	dual cubic & $0.5$ & $4$\\
%	dual diamond&	$\sqrt{2}$& $6$\\
%	dual Laves &	$\sqrt{14}$ & $8$
%\end{tabular}
%\caption{Specifics for intertwined graph topologies of the triply periodic surfaces P, D and G}
%\label{tab:dist_crit}
%\end{table}
\subsection{Complementary cubic lattices}
 In Figure \ref{fig:bilayer} we present the nullity transition for the intertwined cubic networks, displaying yet again the retardation of  the transitions onset for increasing coupling $\lambda_1$. The dual cubic structure was generated by first repeating a unit cell (consisting of points $\bra{0,0,0}$, $\bra{0,0,1}$, $\bra{1,0,0}$, $\bra{0,1,0}$,$\bra{1,1,1}$, $\bra{1,0,1}$, $\bra{0,1,1}$, $\bra{1,1,0}$, connecting those pairs of relative distance $\delta=1$) periodically with the three translation vectors $\vc{a}=i*\bra{1,0,0}$, $\vc{b}=j*\bra{0,1,0}$, $\vc{c}=k*\bra{0,0,1}$ with $i,j,k \in\mathbb{Z} $. The second network is acquired by copying the first structure and shifting it by $\vc{t}=\bra{0.5,0.5,0.5}$.
  \begin{figure}[H]
 	\subfloat[]{\label{fig:bilayer_time_1}	\begin{minipage}[h]{5cm}
 	 \includegraphics[scale=.7]{./Figures_Supplement/21506711/N_275E_450_200000x5e-06mode_pointleaf_alpha_0.1_beta_1.0/eval/combined_radius_time.pdf}
 	 \end{minipage}
 }
 \subfloat[]{\label{fig:bilayer_final_1} 
 	\begin{minipage}[h]{2cm}
 		 \includegraphics[scale=.35]{./Figures_Supplement/21506711/N_275E_450_200000x5e-06mode_pointleaf_alpha_0.1_beta_1.0/eval/network_3d_plot_0.pdf}\\
 		 \includegraphics[scale=.35]{./Figures_Supplement/21506711/N_275E_450_200000x5e-06mode_pointleaf_alpha_0.1_beta_1.0/eval/network_3d_plot_1.pdf}
\end{minipage}} \hfill
 		\subfloat[]{\label{fig:bilayer_time_2}	\begin{minipage}[h]{5cm} \includegraphics[scale=.7]{./Figures_Supplement/21506711/N_275E_450_200000x1e-09mode_pointleaf_alpha_0.1_beta_100000000.0/eval/combined_radius_time.pdf}
 		 \end{minipage}}
 	\subfloat[]{\label{fig:bilayer_final_2}\begin{minipage}{2cm}
 		 \includegraphics[scale=.35]{./Figures_Supplement/21506711/N_275E_450_200000x1e-09mode_pointleaf_alpha_0.1_beta_100000000.0/eval/network_3d_plot_0.pdf}\\
 		 \includegraphics[scale=.35]{./Figures_Supplement/21506711/N_275E_450_200000x1e-09mode_pointleaf_alpha_0.1_beta_100000000.0/eval/network_3d_plot_1.pdf}
\end{minipage} }\\
 		\subfloat[]{\label{fig:bilayer_time_3}	\begin{minipage}[h]{5cm} \includegraphics[scale=.7]{./Figures_Supplement/21506711/N_275E_450_200000x1e-09mode_pointleaf_alpha_1000.0_beta_100000000.0/eval/combined_radius_time.pdf} \end{minipage}}
 	\subfloat[]{\label{fig:bilayer_final_3} \begin{minipage}{2cm}
 		 \includegraphics[scale=.35]{./Figures_Supplement/21506711/N_275E_450_200000x1e-09mode_pointleaf_alpha_1000.0_beta_100000000.0/eval/network_3d_plot_0.pdf}\\
 		 \includegraphics[scale=.35]{./Figures_Supplement/21506711/N_275E_450_200000x1e-09mode_pointleaf_alpha_1000.0_beta_100000000.0/eval/network_3d_plot_1.pdf}
\end{minipage} }\hfill
 		\subfloat[]{\label{fig:bilayer_time_4}	\begin{minipage}[h]{5cm} \includegraphics[scale=.7]{./Figures_Supplement/21506711/N_275E_450_200000x5e-06mode_pointleaf_alpha_1000.0_beta_1.0/eval/combined_radius_time.pdf} \end{minipage}}
 	\subfloat[]{\label{fig:bilayer_final_4} \begin{minipage}{2cm}
 		 \includegraphics[scale=.35]{./Figures_Supplement/21506711/N_275E_450_200000x5e-06mode_pointleaf_alpha_1000.0_beta_1.0/eval/network_3d_plot_0.pdf}\\
 		 \includegraphics[scale=.35]{./Figures_Supplement/21506711/N_275E_450_200000x5e-06mode_pointleaf_alpha_1000.0_beta_1.0/eval/network_3d_plot_1.pdf}
\end{minipage} }
 	\caption{Adaptation Dynamics for a complimentary cubic lattice system and pruned network skeletons. The edge thickness is representative for the relative tube radius $\rho$. \subR{fig:bilayer_time_1}$+$\subR{fig:bilayer_final_1} $\lambda_1=1$, $\lambda_3=0.1$ \subR{fig:bilayer_time_2}$+$\subR{fig:bilayer_final_2} $\lambda_1=10^8$, $\lambda_3=0.1$ \subR{fig:bilayer_time_3}$+$\subR{fig:bilayer_final_3} $\lambda_1=10^8$, $\lambda_3=10^3$ \subR{fig:bilayer_time_4}$+$\subR{fig:bilayer_final_4} $\lambda_1=1$, $\lambda_3=10^3$}\label{fig:bilayer_dynamics}
 \end{figure}
\begin{figure}[H]
	\hspace{-1cm}\subfloat[]{\label{fig:bilayer_aux_3} \includegraphics[scale=1.]{./Figures_Supplement/21572518/sweep_eval/NULLITY_FIT_0.pdf}}
 	\subfloat[]{\label{fig:bilayer_aux_4} \includegraphics[scale=1.]{./Figures_Supplement/21572518/sweep_eval/NULLITY_FIT_1.pdf}}\\
 	\subfloat[]{	\label{fig:bilayer_nullity_c1} \includegraphics[scale=1.]{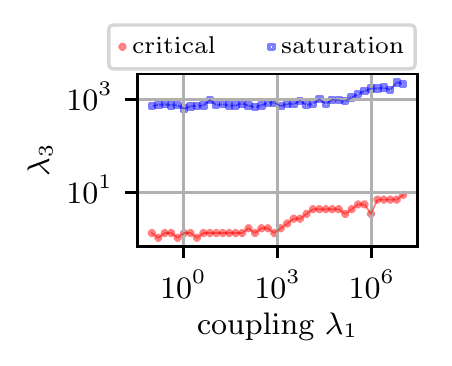}}
 	\subfloat[]{	\label{fig:bilayer_nullity_c2} \includegraphics[scale=1.]{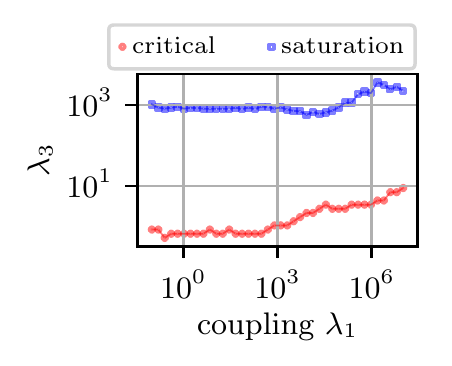}}
 	\caption{Numeric results and analysis of  for a complimentary cubic lattice system: \subR{fig:bilayer_aux_3}+\subR{fig:bilayer_aux_4} Continuous, logarithmic nullity transition in dependency for various coupling $\lambda_1$. Increasing coupling breaks down fluctuation induced nullity.  \subR{fig:bilayer_nullity_c1}$+$\subR{fig:bilayer_nullity_c2} Saturation (blue, squares) and critical values (red circles) in dependency of coupling $\lambda_1$.}\label{fig:bilayer}
\end{figure}
Phenomenologically, the transition resembles an asymmetrical sigmoidal for $\lambda_3 > \lambda_c$, whose saturation value, steepness and x-offset are functions of $\lambda_1$.  Note that, though qualitatively similar, the curves development for increasing $\lambda_1$ is different in the two networks. In particular we observe a significant change of the saturation onset in the second network, see Figure \ref{fig:bilayer_nullity_c1}, \ref{fig:bilayer_nullity_c2}. Next we have listed the systematic $\lambda_1$, $\lambda_3$ of the final stationary state after pruning. In Figure \ref{fig:bilayer_nullity_c1}, \ref{fig:bilayer_nullity_c2} we present the nullity state diagrams as well as the respective outline of their transition zones: first spanning trees, second the onset of redundancy and third the onset of saturation. The colored, dashed boundaries of these zones represent the curves' fits from Figure \ref{fig:bilayer_nullity_c1} and \ref{fig:bilayer_nullity_c1}.
%In Figure \ref{fig:bilayer_aux_3},\ref{fig:bilayer_aux_4} we show dissipation diagrams, presenting the the systems power dissipation ${D=\sum_e \kappa_{ee} \mean{\LP \Phi_e^2}}$ for each network. Note that the systems dissipation is not significantly increased  by an increase of the coupling until extreme values for $\lambda_1$ are reached.  In Figure \ref{fig:bilayer_aux_5},\ref{fig:bilayer_aux_6} we show the networks volume calculated as $V=\sum_e \rho_e^2$ (vessel segments are modelled as cylindrical tubes). We observe here that the tube system collapses for $\lambda_1 > 10^5$ in opposition to the fluctuation induced increase of the systems volume.
In Figure \ref{fig:bilayer_dynamics} we present the numeric results for the systems radii dynamics and plots of the pruned networks for various parameter combinations. An increase in $\lambda_1=\frac{b\bra{\varepsilon-1}}{\pi l \eta L^{\varepsilon+1}}\bra{\frac{\mu}{L^3}}^{-2}$ is decreasing the final radius size $\rho_e$, as it incorporates not only the strength of the repulsive potential but can also be seen as an increase off the systems density by bringing the edges closer to each other.
\subsection{Complementary diamond lattices}
The next segment will contain the gathered results for dual diamond structures where we see the results to be very similar to the cubic structure. The dual structure was generated by first repeating a unit cell (consisting of points $\bra{0,0,0}$,$\bra{0.5,0.5,0.5}$, $\bra{1,0,1}$, $\bra{0,1,1}$, $\bra{1,1,0}$ , connecting those pairs of relative distance $\delta=\sqrt{3}/2$) periodically with the three translation vectors $\vc{a}=i*\bra{1,0,0}$, $\vc{b}=j*\bra{0,1,0}$, $\vc{c}=k*\bra{0,0,1}$ with $i,j,k \in\mathbb{Z}$ and $(i+j+k) mod 2=0$. The second network is acquired by copying the first structure and shifting it by $\vc{t}=\bra{1,1,1}$.
\begin{figure}[H]
  
 	\subfloat[]{\label{fig:bilayer_time_1}	\begin{minipage}[h]{5cm}
 	 \includegraphics[scale=.7]{./Figures_Supplement/22809199/N_141E_214_250000x1e-06mode_pointleaf_alpha_0.1_beta_1.0/eval/combined_radius_time.pdf}
 	 \end{minipage}
 }
 \subfloat[]{\label{fig:bilayer_final_1} 
 	\begin{minipage}[h]{2cm}
 		 \includegraphics[scale=.35]{./Figures_Supplement/22809199/N_141E_214_250000x1e-06mode_pointleaf_alpha_0.1_beta_1.0/eval/network_3d_plot_0.pdf}\\
 		 \includegraphics[scale=.35]{./Figures_Supplement/22809199/N_141E_214_250000x1e-06mode_pointleaf_alpha_0.1_beta_1.0/eval/network_3d_plot_1.pdf}
\end{minipage}} \hfill
 		\subfloat[]{\label{fig:bilayer_time_2}	\begin{minipage}[h]{5cm} \includegraphics[scale=.7]{./Figures_Supplement/22809199/N_141E_214_200000x1e-09mode_pointleaf_alpha_0.1_beta_100000000.0/eval/combined_radius_time.pdf}
 		 \end{minipage}}
 	\subfloat[]{\label{fig:bilayer_final_2}\begin{minipage}{2cm}
 		 \includegraphics[scale=.35]{./Figures_Supplement/22809199/N_141E_214_200000x1e-09mode_pointleaf_alpha_0.1_beta_100000000.0/eval/network_3d_plot_0.pdf}\\
 		 \includegraphics[scale=.35]{./Figures_Supplement/22809199/N_141E_214_200000x1e-09mode_pointleaf_alpha_0.1_beta_100000000.0/eval/network_3d_plot_1.pdf}
\end{minipage} }\\
 		\subfloat[]{\label{fig:bilayer_time_3}	\begin{minipage}[h]{5cm} \includegraphics[scale=.7]{./Figures_Supplement/22809199/N_141E_214_200000x1e-09mode_pointleaf_alpha_1000.0_beta_100000000.0/eval/combined_radius_time.pdf} \end{minipage}}
 	\subfloat[]{\label{fig:bilayer_final_3} \begin{minipage}{2cm}
 		 \includegraphics[scale=.35]{./Figures_Supplement/22809199/N_141E_214_200000x1e-09mode_pointleaf_alpha_1000.0_beta_100000000.0/eval/network_3d_plot_0.pdf}\\
 		 \includegraphics[scale=.35]{./Figures_Supplement/22809199/N_141E_214_200000x1e-09mode_pointleaf_alpha_1000.0_beta_100000000.0/eval/network_3d_plot_1.pdf}
\end{minipage} }\hfill
 		\subfloat[]{\label{fig:bilayer_time_4}	\begin{minipage}[h]{5cm} \includegraphics[scale=.7]{./Figures_Supplement/22809199/N_141E_214_250000x1e-06mode_pointleaf_alpha_1000.0_beta_1.0/eval/combined_radius_time.pdf} \end{minipage}}
 	\subfloat[]{\label{fig:bilayer_final_4} \begin{minipage}{2cm}
 		 \includegraphics[scale=.35]{./Figures_Supplement/22809199/N_141E_214_250000x1e-06mode_pointleaf_alpha_1000.0_beta_1.0/eval/network_3d_plot_0.pdf}\\
 		 \includegraphics[scale=.35]{./Figures_Supplement/22809199/N_141E_214_250000x1e-06mode_pointleaf_alpha_1000.0_beta_1.0/eval/network_3d_plot_1.pdf}
\end{minipage} }
 	\caption{Adaptation Dynamics for a complimentary diamond graph system and pruned network skeletons. The edge thickness is representative for the relative tube radius $\rho$. \subR{fig:bilayer_time_1}$+$\subR{fig:bilayer_final_1} $\lambda_1=1$, $\lambda_3=0.1$ \subR{fig:bilayer_time_2}$+$\subR{fig:bilayer_final_2} $\lambda_1=10^8$, $\lambda_3=0.1$ \subR{fig:bilayer_time_3}$+$\subR{fig:bilayer_final_3} $\lambda_1=10^8$, $\lambda_3=10^3$ \subR{fig:bilayer_time_4}$+$\subR{fig:bilayer_final_4} $\lambda_1=1$, $\lambda_3=10^3$}\label{fig:bilayer_dynamics}
 \end{figure}
\begin{figure}[H]
	\hspace{-1cm}\subfloat[]{\label{fig:D_3} \includegraphics[scale=1.]{./Figures_Supplement/22926223/sweep_eval/NULLITY_FIT_0.pdf}}
 	\subfloat[]{\label{fig:D_4} \includegraphics[scale=1.]{./Figures_Supplement/22926223/sweep_eval/NULLITY_FIT_1.pdf}}\\
 	\subfloat[]{	\label{fig:D_nullity_c1} \includegraphics[scale=1.]{./Figures_Supplement/22926223/sweep_eval/fit_critical_saturation_0.pdf}}
 	\subfloat[]{	\label{fig:D_nullity_c2} \includegraphics[scale=1.]{./Figures_Supplement/22926223/sweep_eval/fit_critical_saturation_1.pdf}}
 	\caption{Numeric results and analysis for a complimentary diamond graph system: \subR{fig:bilayer_aux_3}+\subR{fig:bilayer_aux_4} Continuous, logarithmic nullity transition in dependency for various coupling $\lambda_1$. Increasing coupling breaks down fluctuation induced nullity.  \subR{fig:bilayer_nullity_c1}$+$\subR{fig:bilayer_nullity_c2} Saturation (blue, squares) and critical values (red circles) in dependency of coupling $\lambda_1$.}\label{fig:bilayer_D}
\end{figure}
% \begin{figure}[H]
% \vspace{-2cm}
% 	\subfloat[]{\label{fig:bilayer_D_1} \includegraphics[scale=1.]{./Figures_Supplement/22926223/sweep_eval/NULLITY_MATRIX_0_extended.pdf}}
% 	\subfloat[]{\label{fig:bilayer_D_2} \includegraphics[scale=1.]{./Figures_Supplement/22926223/sweep_eval/NULLITY_MATRIX_1_extended.pdf}}\\
% 	\subfloat[]{\label{fig:bilayer_D_3} \includegraphics[scale=1.]{./Figures_Supplement/22926223/sweep_eval/DISS_MATRIX_0.pdf}}
% 	\subfloat[]{\label{fig:bilayer_D_4} \includegraphics[scale=1.]{./Figures_Supplement/22926223/sweep_eval/DISS_MATRIX_1.pdf}}\\
% 	\subfloat[]{\label{fig:bilayer_D_5} \includegraphics[scale=1.]{./Figures_Supplement/22926223/sweep_eval/VOL_MATRIX_0.pdf}}
% 	\subfloat[]{\label{fig:bilayer_D_6} \includegraphics[scale=1.]{./Figures_Supplement/22926223/sweep_eval/VOL_MATRIX_1.pdf}}
% 	\caption{Numeric results and analysis for a 'dual' diamond graph system: \subR{fig:bilayer_aux_1}$+$\subR{fig:bilayer_aux_2}Nullity $\varrho$ state diagrams with borders of the transition zones plotted as dashed lines( red $=$ onset of nullity transition, black $=$ onset of saturation) \subR{fig:bilayer_aux_3}$+$\subR{fig:bilayer_aux_4}Dissipation diagrams, coupling $\lambda_1$ and fluctuation $\lambda_3$ are not majorly affecting the systems dissipation \subR{fig:bilayer_aux_5}$+$\subR{fig:bilayer_aux_6} Volume diagrams, we observe an increase of V for increased $\lambda_3$, a collapse is occuring for increased $\lambda_1$.}\label{fig:bilayer2}
% \end{figure}
\subsection{Complementary Laves graphs}
The next segment will contain the gathered results for dual Laves structures where we see the results as well to be very similar to the cubic structure. The dual structure was generated by first repeating a unit cell (consisting of points $\bra{0,0,0}$,$\bra{1,1,0}$, $\bra{1,2,1}$, $\bra{0,3,1}$, $\bra{2,2,2}$, $\bra{3,3,2}$, $\bra{3,0,3}$ , $\bra{2,1,3}$, connecting those pairs of relative distance $\delta=\sqrt{2}$) periodically with the three translation vectors $\vc{a}=i*\bra{4,0,0}$, $\vc{b}=j*\bra{0,4,0}$, $\vc{c}=k*\bra{0,0,4}$ with $i,j,k \in\mathbb{Z}$. The second network is acquired mirroring in order to create the opposing chirality of the first structure, i.e. $\vc{a}\rightarrow -\vc{a}$, and shifting it by $\vc{t}=\bra{3,2,0}$.
\begin{figure}[H]

 	\subfloat[]{\label{fig:bilayer_time_1}	\begin{minipage}[h]{5cm}
 	 \includegraphics[scale=.7]{./Figures_Supplement/22809169/N_206E_259_250000x1e-06mode_pointleaf_alpha_0.1_beta_1.0/eval/combined_radius_time.pdf}
 	 \end{minipage}
 }
 \subfloat[]{\label{fig:bilayer_final_1} 
 	\begin{minipage}[h]{2cm}
 		 \includegraphics[scale=.35]{./Figures_Supplement/22809169/N_206E_259_250000x1e-06mode_pointleaf_alpha_0.1_beta_1.0/eval/network_3d_plot_0.pdf}\\
 		 \includegraphics[scale=.35]{./Figures_Supplement/22809169/N_206E_259_250000x1e-06mode_pointleaf_alpha_0.1_beta_1.0/eval/network_3d_plot_1.pdf}
\end{minipage}} \hfill
 		\subfloat[]{\label{fig:bilayer_time_2}	\begin{minipage}[h]{5cm} \includegraphics[scale=.7]{./Figures_Supplement/22809169/N_206E_259_200000x1e-09mode_pointleaf_alpha_0.1_beta_100000000.0/eval/combined_radius_time.pdf}
 		 \end{minipage}}
 	\subfloat[]{\label{fig:bilayer_final_2}\begin{minipage}{2cm}
 		 \includegraphics[scale=.35]{./Figures_Supplement/22809169/N_206E_259_200000x1e-09mode_pointleaf_alpha_0.1_beta_100000000.0/eval/network_3d_plot_0.pdf}\\
 		 \includegraphics[scale=.35]{./Figures_Supplement/22809169/N_206E_259_200000x1e-09mode_pointleaf_alpha_0.1_beta_100000000.0/eval/network_3d_plot_1.pdf}
\end{minipage} }\\
 		\subfloat[]{\label{fig:bilayer_time_3}	\begin{minipage}[h]{5cm} \includegraphics[scale=.7]{./Figures_Supplement/22809169/N_206E_259_200000x1e-09mode_pointleaf_alpha_1000.0_beta_100000000.0/eval/combined_radius_time.pdf} \end{minipage}}
 	\subfloat[]{\label{fig:bilayer_final_3} \begin{minipage}{2cm}
 		 \includegraphics[scale=.35]{./Figures_Supplement/22809169/N_206E_259_200000x1e-09mode_pointleaf_alpha_1000.0_beta_100000000.0/eval/network_3d_plot_0.pdf}\\
 		 \includegraphics[scale=.35]{./Figures_Supplement/22809169/N_206E_259_200000x1e-09mode_pointleaf_alpha_1000.0_beta_100000000.0/eval/network_3d_plot_1.pdf}
\end{minipage} }\hfill
 		\subfloat[]{\label{fig:bilayer_time_4}	\begin{minipage}[h]{5cm} \includegraphics[scale=.7]{./Figures_Supplement/22809169/N_206E_259_250000x1e-06mode_pointleaf_alpha_1000.0_beta_1.0/eval/combined_radius_time.pdf} \end{minipage}}
 	\subfloat[]{\label{fig:bilayer_final_4} \begin{minipage}{2cm}
 		 \includegraphics[scale=.35]{./Figures_Supplement/22809169/N_206E_259_250000x1e-06mode_pointleaf_alpha_1000.0_beta_1.0/eval/network_3d_plot_0.pdf}\\
 		 \includegraphics[scale=.35]{./Figures_Supplement/22809169/N_206E_259_250000x1e-06mode_pointleaf_alpha_1000.0_beta_1.0/eval/network_3d_plot_1.pdf}
\end{minipage} }
 	\caption{Adaptation Dynamics for a complimentary Laves graph system and pruned network skeletons. The edge thickness is representative for the relative tube radius $\rho$. \subR{fig:bilayer_time_1}$+$\subR{fig:bilayer_final_1} $\lambda_1=1$, $\lambda_3=0.1$ \subR{fig:bilayer_time_2}$+$\subR{fig:bilayer_final_2} $\lambda_1=10^8$, $\lambda_3=0.1$ \subR{fig:bilayer_time_3}$+$\subR{fig:bilayer_final_3} $\lambda_1=10^8$, $\lambda_3=10^3$ \subR{fig:bilayer_time_4}$+$\subR{fig:bilayer_final_4} $\lambda_1=1$, $\lambda_3=10^3$}\label{fig:bilayer_dynamics}
 \end{figure}
\begin{figure}[H]
	\hspace{-1cm}\subfloat[]{\label{fig:D_3} \includegraphics[scale=1.]{./Figures_Supplement/22868425/sweep_eval/NULLITY_FIT_0.pdf}}
 	\subfloat[]{\label{fig:D_4} \includegraphics[scale=1.]{./Figures_Supplement/22868425/sweep_eval/NULLITY_FIT_1.pdf}}\\
 	\subfloat[]{	\label{fig:D_nullity_c1} \includegraphics[scale=1.]{./Figures_Supplement/22868425/sweep_eval/fit_critical_saturation_0.pdf}}
 	\subfloat[]{	\label{fig:D_nullity_c2} \includegraphics[scale=1.]{./Figures_Supplement/22868425/sweep_eval/fit_critical_saturation_1.pdf}}
 	\caption{Numeric results and analysis for a 'dual' Laves graph system: \subR{fig:bilayer_aux_3}+\subR{fig:bilayer_aux_4} Continuous, logarithmic nullity transition in dependency for various coupling $\lambda_1$. Increasing coupling breaks down fluctuation induced nullity.  \subR{fig:bilayer_nullity_c1}$+$\subR{fig:bilayer_nullity_c2} Saturation (blue, squares) and critical values (red circles) in dependency of coupling $\lambda_1$.}\label{fig:bilayer_D}
\end{figure}
% \begin{figure}[H]
% \vspace{-2cm}
% 	\subfloat[]{\label{fig:bilayer_D_1} \includegraphics[scale=1.]{./Figures_Supplement/22868425/sweep_eval/NULLITY_MATRIX_0_extended.pdf}}
% 	\subfloat[]{\label{fig:bilayer_D_2} \includegraphics[scale=1.]{./Figures_Supplement/22868425/sweep_eval/NULLITY_MATRIX_1_extended.pdf}}\\
% 	\subfloat[]{\label{fig:bilayer_D_3} \includegraphics[scale=1.]{./Figures_Supplement/22868425/sweep_eval/DISS_MATRIX_0.pdf}}
% 	\subfloat[]{\label{fig:bilayer_D_4} \includegraphics[scale=1.]{./Figures_Supplement/22868425/sweep_eval/DISS_MATRIX_1.pdf}}\\
% 	\subfloat[]{\label{fig:bilayer_D_5} \includegraphics[scale=1.]{./Figures_Supplement/22868425/sweep_eval//VOL_MATRIX_0.pdf}}
% 	\subfloat[]{\label{fig:bilayer_D_6} \includegraphics[scale=1.]{./Figures_Supplement/22868425/sweep_eval/VOL_MATRIX_1.pdf}}
% 	\caption{Numeric results and analysis for a 'dual' Laves graph system: \subR{fig:bilayer_aux_1}$+$\subR{fig:bilayer_aux_2}Nullity $\varrho$ state diagrams with borders of the transition zones plotted as dashed lines( red $=$ onset of nullity transition, black $=$ onset of saturation) \subR{fig:bilayer_aux_3}$+$\subR{fig:bilayer_aux_4}Dissipation diagrams, coupling $\lambda_1$ and fluctuation $\lambda_3$ are not majorly affecting the systems dissipation \subR{fig:bilayer_aux_5}$+$\subR{fig:bilayer_aux_6} Volume diagrams, we observe an increase of V for increased $\lambda_3$, a collapse is occuring for increased $\lambda_1$.}\label{fig:bilayer2}
% \end{figure}

\newpage
\input{./Sections_Supplement/appendix_e}

\bibliography{../../../lib2}

\end{document}
